# Supplementary material for: Stability of Aggregation Graph Neural Networks
Source: arXiv:2207.03678 source file (2023-08-23)
Supplement: Supplementary file 1 [file appendix_HsFrechet.tex]

%!TEX root =../compiler_paper.tex




%
%%%--------------------------------------------------------------------------------------------------------------------------------
%%%------------------------ FRECHET DERIVATIVE OF LIPSCHITZ FUNCTIONS -------------------------------
%%%---------------------------------------------------------------------------------------------------------------------------------
%
%\section{Fr\'echet Derivative of Lipschitz Functions}
%\label{appendix_FDLF}
%
%
%
%%%%%%%%%%%%%%%%%%%%%%%%%%%%%%%%%%%%%%%%%%%%%%%%%
%%%%%%%%%%%%%%%%% THEOREM %%%%%%%%%%%%%%%%%%%%%%%%%%
%%%%%%%%%%%%%%%%%%%%%%%%%%%%%%%%%%%%%%%%%%%%%%%%%
%
%
%\begin{theorem}\label{theorem:FDLF}
%
%Let $\bbF: \ccalV \to \ccalU$ a Lipschitz map between two Banach spaces $\ccalV$ and $\ccalU$ with Lipschitz constant $L_{0}$. Let $\bbD_{\bbF\vert\bbS}(\bbS)$ be the Fr\'echet derivative of $\bbF$ at $\bbS\in\End{V}$. Then, if $\bbD_{\bbF\vert\bbS}(\bbS)$ exists we have that
%%
%%
%%
%\begin{equation}
%\left\Vert
%                \bbD_{\bbF\vert\bbS}(\bbS)
%\right\Vert
%                \leq 
%                       L_{0}
%\end{equation}
%%
%%
%%
%
%\end{theorem}
%
%\begin{proof}
%
%We start taking into account the definition of the Fr\'echet derivative of $\bbF(\bbS)$ we have
%
%%
%%
%\begin{equation}
%\lim_{\Vert \boldsymbol{\xi}\Vert\to 0}
%                                                    \frac{
%                                                             \left\Vert
%                                                                    \bbF(\bbS+\boldsymbol{\xi})-\bbF(\bbS)-\bbD_{\bbF\vert\bbS}(\bbS)\{ \boldsymbol{\xi} \}
%                                                             \right\Vert
%                                                     }
%                                                     {
%                                                        \Vert \boldsymbol{\xi} \Vert 
%                                                     }
%                                                     =
%                                                       0
%\end{equation}
%%
%%
%
%Then, we have that
%
%%
%%
%\begin{equation}\label{eq:appendix1}
%\left\Vert
%                \frac{
%                 \bbF(\bbS+\boldsymbol{\xi})-\bbF(\bbS)
%                }
%                {
%                \Vert \boldsymbol{\xi} \Vert
%                }
%                -
%                \frac{
%                \bbD_{\bbF\vert\bbS}(\bbS)\{ \boldsymbol{\xi} \}
%                }
%                {
%                \Vert \boldsymbol{\xi} \Vert
%                }
%\right\Vert
%                =
%                \epsilon\left( \Vert \boldsymbol{\xi}\Vert\right)
%\end{equation}
%%
%%
%
%with $ \epsilon\left( \Vert \boldsymbol{\xi}\Vert\right)\to 0$ as $ \Vert \boldsymbol{\xi}\Vert\to 0$ and  $ \epsilon\left( \Vert \boldsymbol{\xi}\Vert\right)\geq 0$. Now, from eqn.~(\ref{eq:appendix1})  and using the reverse triangle inequality we obtain the following expression
%
%%
%%
%\begin{equation}
%\left\Vert                
%                \frac{
%                \bbD_{\bbF\vert\bbS}(\bbS)\{ \boldsymbol{\xi} \}
%                }
%                {
%                \Vert \boldsymbol{\xi} \Vert
%                }
%\right\Vert
%               -
%\left\Vert
%                \frac{
%                 \bbF(\bbS+\boldsymbol{\xi})-\bbF(\bbS)
%                }
%                {
%                \Vert \boldsymbol{\xi} \Vert
%                }
%\right\Vert                
%                \leq
%                \epsilon\left( \Vert \boldsymbol{\xi}\Vert\right).
%\end{equation}
%%
%%
%
%Therefore, we have 
%
%%
%%
%\begin{equation}
%\left\Vert                
%                \frac{
%                \bbD_{\bbF\vert\bbS}(\bbS)\{ \boldsymbol{\xi} \}
%                }
%                {
%                \Vert \boldsymbol{\xi} \Vert
%                }
%\right\Vert
%               \leq
%\left\Vert
%                \frac{
%                 \bbF(\bbS+\boldsymbol{\xi})-\bbF(\bbS)
%                }
%                {
%                \Vert \boldsymbol{\xi} \Vert
%                }
%\right\Vert ,                
%\end{equation}
%%
%%
%
%and taking into account that $\bbF(\bbS)$ is Lipschitz with constant $L_{0}$ we obtain
%
%%
%%
%\begin{equation}
%\left\Vert
%               \bbD_{\bbF\vert\bbS}(\bbS)\{ \boldsymbol{\xi} \}
%\right\Vert
%               \leq
%                     L_{0} \Vert\boldsymbol{\xi}\Vert,
%\end{equation}
%%
%%
%
%which considering the operator norm, leads to $\bbD_{\bbF\vert\bbS}(\bbS)\leq L_{0}$.
%
%\end{proof}
